# Supplementary material for: ControlRoom3D: Room Generation using Semantic Proxy Rooms
Source: arXiv:2312.05208 source file (2023-12-08)

without SAM masks

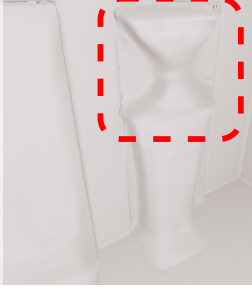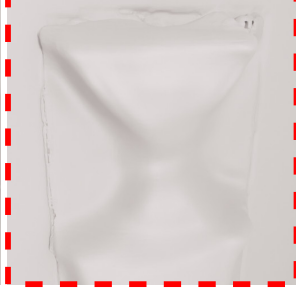

with SAM masks

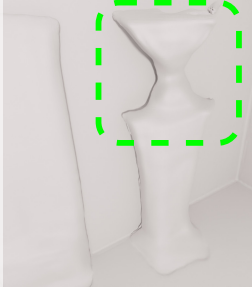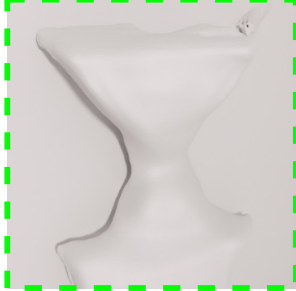

without normal loss

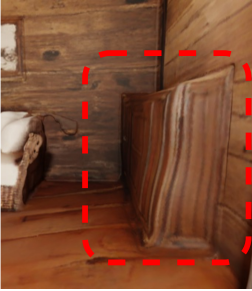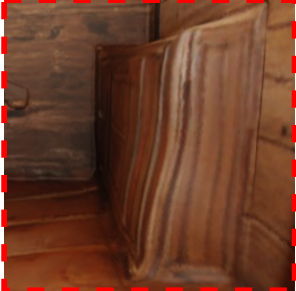

with normal loss

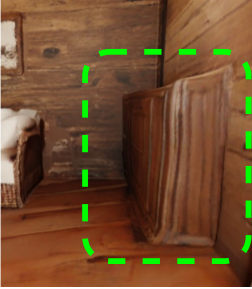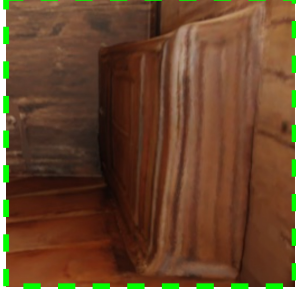

Supplement: Supplementary file 1 [file supp_depth.pdf]
